# Supplementary material for: Cross-View Completion Models are Zero-shot Correspondence Estimators
Source: arXiv:2412.09072 source file (2024-12-12)
Supplement: Supplementary file 13 [file depth_ablation.tex]

\begin{table}[t!]
\centering
\resizebox{\linewidth}{!}{

\begin{tabular}{c|c|c|ccc|c}
\toprule
Depth & \multicolumn{2}{c|}{Aggregation} & 
\multirow[c]{2}{*}{AbsRel$\downarrow$} &
\multirow[c]{2}{*}{SqRel$\downarrow$} &
\multirow[c]{2}{*}{RMSE$\downarrow$}  &
\multirow[c]{2}{*}{\textbf{$\delta_1$}$\uparrow$}\\
\cline{2-3}
head &  $\mathcal{F}_{attn}$ & $\mathcal{F}_{feat}$ &&&&\\
\midrule
\midrule
DPT  & \ding{55} & \ding{55} & 0.102 & 0.767 & 4.351 & 0.903 \\
Aggregator & \ding{51} & \ding{55} & 0.150 & 1.235 & 5.515& 0.808 \\
Aggregator  & \ding{55} & \ding{51} & 0.092 & 0.650 & 4.218 & 0.910\\
\midrule
Aggregator &\ding{51}&\ding{51}&  \textbf{0.090} & \textbf{0.637 }& \textbf{4.128} & \textbf{0.915}\\
\bottomrule
		\end{tabular}
	}
    \vspace{-5pt}
    \caption{\textbf{Ablation studies on the KITTI Dataset.}
    }
    \vspace{-10pt}
    \label{suptab:depth_abl}
\end{table}
